# Supplementary material for: Taste More, Taste Better: Diverse Data and Strong Model Boost Semi-Supervised Crowd Counting
Source: arXiv:2503.17984 source file (2025-03-23)
Supplement: Supplementary file 1 [file X_suppl.tex]

\clearpage
\setcounter{page}{1}
\maketitlesupplementary

\section{Mathematical Definitions of MAE and RMSE Metrics}

The MAE and RMSE are defined as follows:
\begin{equation}
    \label{eq:mae_rmse}
    \begin{split}
        \text{MAE} & = \frac{1}{N_i} \sum_{i=1}^{N_i} |C_i^{g t} - \hat{C}_i|, \\
        \text{RMSE} & = \sqrt{\frac{1}{N_i} \sum_{i=1}^{N_i} (C_i^{g t} - \hat{C}_i)^2}.
    \end{split}
\end{equation}
where $N_i$ is the number of images, $C_i^{g t}$ is the ground truth count, and $\hat{C}_i$ is the estimated count.

\section{Detailed study of the weight decay speed}

We study the impact of the weight decay speed $T^{\text{inpw}}$ on the JHU-Crowd++ dataset with 5\% labeled data. The influence of $T^{\text{inpw}}$ on the MAE and RMSE is shown in \Cref{fig:abl_inpw}. 
We train and test TMTB with different $T^{\text{inpw}}$ values ranging from $80$ to $120$. 
The results show that both MAE and RMSE decrease as $T^{\text{inpw}}$ increases from $80$ to $100$. 
However, when $T^{\text{inpw}}$ is greater than $100$, the performance begins to degrade. 
Therefore, we set $T^{\text{inpw}}$ to $100$ in experiments, which achieves the best performance.

\begin{figure}
    \centering
    \includegraphics[width=0.9\linewidth]{figure/T^inpw/Tinpw.png}
    \caption{The impact of the weight decay speed $T^{\text{inpw}}$ on the JHU-Crowd++ dataset with 5\% labeled data.}
    \label{fig:abl_inpw}
    \vspace{-0.2 cm}
\end{figure}

\section{Detailed study of the number of warm-up epochs}

We calculate $\lambda_{w}$ based on training epoch $t$ and pre-defined warm-up epoch $T^{w}$ as $\lambda_{w}= e^{-5.0 * (1.0-t/T^{w})^2}$, when $t < T^{w}$. $\lambda_{w}$ is set to $1.0$ when $t \geq T^{w}$. \Cref{tab:abl_warmup} presents the experiments on 10\% ShanghaiTech A to find optimal $T^{w}$. 

\begin{table}
    \caption{The impact of the number of warm-up epochs $T^{w}$ on the ShanghaiTech A dataset with 10\% labeled data.}
    \label{tab:abl_warmup}
    \centering
    \begin{tabular}{l|cc}
        $T^{w}$ & MAE & RMSE \\
        \midrule
        0 & 70.0 & 121.1 \\
        5 & 70.6 & 116.2 \\
        10 & 66.0 & 113.6 \\
        20 & \textbf{65.7} & \textbf{110.4} \\
        30 & 68.5 & 113.1 \\
        40 & 67.4 & 114.2 \\
        60 & 70.6 & 118.4 \\
        80 & 70.2 & 120.5 \\
    \end{tabular}
\end{table}

\section{Text Prompts in Inpainting}

We generate some positive text prompts to inpaint the images with diverse backgrounds and scenarios. The prompts are generated by large language models (LLMs), GPT-4o~\cite{openai2024gpt4ocard}. 

All inpainting processes share the same negative prompt. For the balance of diversity and quality, we do not forbid drawing extra people. The negtive text prompt we employed is:
\begin{quote}
    disfigured face, broken limbs, deformed body parts
\end{quote}

And we design the positive prompts with diverse scenarios containing plants or animals. All used postive prompts are listed in \Cref{tab:prompts}. Note that, updating the prompts while inpainting is also available, and we employ the fixed database for simplicity.

\begin{table*}
\caption{Positive prompts that we used in inpainting.}
\label{tab:prompts}
\centering
\begin{tabular}{|l|}
\hline
\multirow{2}{*}{\textbf{Positive Prompts}} \\ \\ \hline 
sunset over mountains, a lone eagle soaring, vibrant colors \\ \hline
ancient forest, misty atmosphere, deer grazing among trees \\ \hline
futuristic city skyline, neon-lit drones flying, cyberpunk style \\ \hline
serene beach, seashells scattered on the sand, gentle waves \\ \hline
snowy village, a fox prowling near cozy cabins, northern lights above \\ \hline
bustling marketplace, exotic fruits and spices, colorful fabrics swaying \\ \hline
abandoned castle, ivy-covered walls, crows perched on towers \\ \hline
desert landscape, cacti scattered, a lone lizard basking in the sun \\ \hline
underwater world, coral reefs teeming with fish, jellyfish drifting \\ \hline
enchanted garden, blooming roses, butterflies fluttering around \\ \hline
rainy city street, puddles reflecting streetlights, stray cat in the alley \\ \hline
starry night sky, a full moon shining, an owl perched on a tree \\ \hline
autumn forest, falling leaves in warm tones, a squirrel gathering acorns \\ \hline
medieval town square, horses tied to a post, pigeons pecking on cobblestones \\ \hline
tropical jungle, dense foliage, a parrot perched on a branch \\ \hline
twilight in the mountains, calm lake with lily pads, fireflies glowing \\ \hline
bustling urban park, tall trees with squirrels, children flying kites \\ \hline
ancient ruins, crumbling stone with moss, a snake slithering through the grass \\ \hline
futuristic lab, clean and sterile with robotic arms, plants growing in glass chambers \\ \hline
rustic farmhouse, golden wheat fields swaying, a scarecrow standing tall \\ \hline
\end{tabular}
\end{table*}

\section{Further Discussion of Architectures}

\begin{figure}
    \centering
    \includegraphics[width=0.9\linewidth]{figure/smart_mamba/mamba.jpg}
    \caption{2D-Selective-Scan (SS2D) helps the establishment of global receptive fields. Green boxes indicate the query image patch, with patch opacity representing the degree of information loss.}
    \label{fig:cute_mamba}
\end{figure}

In \Cref{fig:cute_mamba}, we visualize the 2D-Selective-Scan mechanism of VMamba~\cite{liu2024vmambavisualstatespace}, which benefits the modeling of global context. The scanning operation in S6 fits well with NLP tasks, while it faces a challenge when applied to vision data. The 2D-Selective-Scan is proposed to adapt S6 in Mamba~\cite{gu2024mambalineartimesequencemodeling} to vision data. SS2D consists of three steps: cross-scan, selective scanning with S6, and cross-merge. SS2D unfolds input patches of an image into sequences along four traversal paths (\ie, Cross-Scan), and processes each sequence with a separate S6 block. After processing, the four sequences are reshaped and the resultant sequences are merged to form the output map (\ie, Cross-Merge). As shown in \Cref{fig:cute_mamba}, SS2D enables every pixel in the image to integrate information from other pixels in four directions, facilitating the establishment of global receptive fields, which is necessary for counting in adverse scenarios. 

\begin{figure}
    \centering
    \subfloat[Image]{\includegraphics[width=0.45\linewidth]{figure/smart_mamba/origin.png}}
    \hfill
    \subfloat[CNN]{\includegraphics[width=0.45\linewidth]{figure/smart_mamba/cnn_den.png}} \\
    \subfloat[CNN\&Transformer]{\includegraphics[width=0.45\linewidth]{figure/smart_mamba/cnnt_den.png}}
    \hfill
    \subfloat[VSSM]{\includegraphics[width=0.45\linewidth]{figure/smart_mamba/vssm_den.png}}
    \caption{Predicted density maps. For the \textcolor[HTML]{00FF9C}{green} bounding box, both CNNs and CNN with Transformer overfit to local texture information, generating nonexistent prediction. For the \textcolor[HTML]{FF0000}{red} bounding box, CNN with Transformer makes extremely erroneous predictions on regions with a strong contrast to the scene. For the \textcolor[HTML]{FFC000}{yellow} bounding box, CNN and CNN with Transformer make inaccurate predictions in low-light regions.}
    \label{fig:archs_den}
\end{figure}

We visualize the density maps predicted by different architectures in \Cref{fig:archs_den}. When facing low-light and adverse scenarios, VSSM still shows great capacity of capturing context features.
